# Supplementary material for: Towards Effective Semantic OOD Detection in Unseen Domains: A Domain Generalization Perspective
Source: arXiv:2309.10209 source file (2023-09-18)
Supplement: Supplementary file 1 [file appendix.tex]

% \subsection{Notations.}
% For clear interpretation, we list the notations used in this paper and their corresponding explanation shown in Table \ref{tab:notations}.
% \begin{table}[h!]
%     \centering
%     \caption{Important notations and corresponding descriptions.}
%     \begin{tabular}{c|p{2.4in}}
%        \toprule
%         \textbf{Notations} & \textbf{Descriptions} \\
%         \midrule
%         $\mathcal{D}$ & entire dataset \\
%         $\mathcal{E}, E, e$ & set of domain labels, number of all domains, index of domains \\
%         $\mathcal{E}_{tr},\mathcal{E}_{te}$ & set of training and testing domains\\
%         $\mathcal{D}_{tr}, \mathcal{D}_{te}$ & training and testing datasets\\
%         $E_{tr}, E_{te}$ & numbers of training and testing domains\\
%         $\mathcal{D}^e, |\mathcal{D}^e|$ & data of domain $e$, size of data of domain $e$  \\
%         $\mathbf{x},y$ &  data instance and its label\\
%         $\mathcal{X}$ & feature space \\
%         $\mathcal{Y}_{tr}, \mathcal{Y}_{te}$ & label spaces of training and testing datasets \\
%         $K$ & total number of training classes \\
%         $y_{InD}, y_{OOD}$ & labels of testing data \\
%         $f$ & the predictor \\
%         $g,h$ & featurizer and classifier of the predictor $f$\\
%         $\omega$ & OOD detector \\
%         $\boldsymbol{\theta}, \boldsymbol{\theta}_g, \boldsymbol{\theta}_h$ & parameters of the predictor, the fraturizer and the classifier \\
%         $\Theta$ & parameter space\\
%         $G$ & the transformation model\\
%         $E_s, E_v, D$ & semantic encoder, the variation encoder, and the decoder\\
%         $\mathcal{S, V}$ & latent semantic and variation spaces\\
%         $\mathbf{s}, \mathbf{v}$ & semantic and variation factors\\
%         $R_{DG}$ & the domain generalization regularizer\\
%         $d$ & distance metrics\\
%         $R_{OOD}$ & the OOD regularizer\\
%         $\lambda_1,\lambda_2$ & mixing parameters\\
%         $\hat{\mathbf{s}}$ & semantic factors after mixing up\\
%         $\hat{\mathbf{x}}$ & generated pseudo-OOD instance\\
%         $\mathcal{D}_{pseudo}$ & dataset of pseudo-OODs\\
%         $\xi$ & empirical threshold qualifying pseudo-OODs\\
%         $\mathbf{x}_{in},y_{InD}$ & InD instances in the training dataset\\
%         $\mathbf{x}_{out},y_{OOD}$ & pseudo-OOD instances\\
%         $m_{in}, m_{out}$ & margins regularizing InD and pseudo-OOD energy scores\\
%         $E_g$ & energy function\\
%         $T$ & temperature parameter\\
%         $\beta_1,\beta_2$ & Lagrangian multipliers (dual variables)\\
%         $\gamma_1,\gamma_2$ & margins of the two regularizers\\
%         $\eta_p,\eta_{dg},\eta_{ood}$ & learning rates of primal and dual parameters\\
%        \bottomrule
%     \end{tabular}
%     \label{tab:notations}
% \end{table}



% \subsection{Architecture of the Transformation Model $G$ and the Predictor $f$.}
% % All the images are resized to 224$\times$224. 
% The semantic encoder $E_s$ is made of four convolution layers. The first one has 64 filters, and each of the others has 128 filters. The kernel sizes are (7,7), (4,4), (3,3), and (3,3) for layers 1-4, respectively. The stride of the second layer is (2,2), and the stride of all the other layers is (1,1). The activation function of the first three layers is ReLU. The last convolution layer does not have an activation function. The variation encoder $E_v$ is made of 6 convolution layers, and there is an adaptive average pooling layer with output size 1 between the last two convolution layers. The numbers of filters are 64, 128, 256, 256, 256, and 2 for the convolution layers, respectively. The kernel sizes are (7,7), (4,4), (4,4), (4,4), (4,4), (1,1). And the strides are (1,1), (2,2), (2,2), (2,2), (2,2), (1,1). The activation function of the first five layers is ReLU. The last convolution layer does not have an activation function. The decoder $D$ is made of 4 convolution layers followed by an average pooling layer whose kernel size is 3, stride is 2, and padding is [1,1]. The numbers of filters of the convolution layers are 64, 128, 256, 1, respectively. The kernel sizes are (4,4) for the first three convolution layers and (1,1) for the fourth convolution layer. The strides are (2,2) for the first three convolution layers and (1,1) for the fourth convolution layer. The first three convolution layers' activation functions are LeakyReLU. The other layers do not have activation functions. The training of $G$ is an end-to-end training.
% As for the predictor $f$, $g$ is Resnet50 \cite{he2016deep}, and $h$ is a fully connected layer with input size 2048 and output size $K$.

% More transformed image examples are shown in Figure \ref{fig:transformed-images}.

% \begin{figure*}[t]
%     \centering
%     \includegraphics[width=0.8\linewidth]{images/transformation.png}
%     \caption{More transformed image examples generated using $G$ with randomly sampled variation factors.
%     }
%     \label{fig:transformed-images}
% \end{figure*}


% \subsection{Training $G$}

% \subsection{Detailed Experimental Settings.}
% \subsubsection{Environment and Experiment Setup.}
% The environment we used: Python: 3.9.13, PyTorch: 1.12.1, Torchvision: 0.13.1, CUDA: 11.6, CUDNN: 8302, NumPy: 1.23.1, PIL: 9.2.0.
% Experiment setup: Our experimental framework, tailored for semantic OOD detection across domains, deviates from the conventional setups for OOD detection and domain generalization. Uniquely, in our configuration, the OOD samples are always sourced from an unseen test domain. For each dataset, we designated one class as OOD and iterate our experiments with different randomly chosen OOD classes until a minimum of 40\% of classes have been designated as OOD. To further mitigate the impact of randomness, each set of experiments is conducted in two separate trials with different seeds. The results reported in the paper represent mean and standard error across these trials and all OOD class choices. Furthermore, given the multiple OOD detection methods evaluated in this study, and in an effort to present the results in a concise manner, for the OOD detection performance we report the averaged values across all test domains unless specified otherwise.

% \subsubsection{Model Selection.} Commonly used model selection strategies include training-domain validation, leave-one-domain-out cross-validation, and test-domain validation. Training-domain validation holds out a portion of the training data as the validation set, but essentially, it assumes that the test domain adheres to the same distribution as the training domains, which contradicts the concept of domain generalization. Test-domain validation uses part of the test set for model selection, but in practice, we typically lack any information about the target domain. Leave-one-domain-out cross-validation utilizes a held-out training domain as a validation set. This strategy presumes that training and test domains follow a meta-distribution over domains, which more closely aligns with real-world scenarios.

% \subsubsection{Hyperparameter Search.}
% Considering both the experimental framework and the practical considerations related to experiment execution time, we carried out a random search of 20 trials over the hyperparameter distribution for each algorithm and test domain. To be more specific, we partitioned the data from each domain into an 80-20 split. The larger portion was designated for training and evaluation, while the smaller was used for hyperparameter selection.
% The detailed hyperparameters space and their corresponding default values are specified in Table \ref{tab:hyperparamesters}, other hyperparameters (\textit{e.g.,} learning rate, weight decay, \textit{etc.}) that are not listed in this table are left unchanged from the DomainBed framework.

% \begin{table}[h!]
%     \centering
%     \caption{Hyperparameters for \sysname{} in different datasets.}
%     \begin{tabular}{c|c|c|c}
%     \toprule
%     \textbf{Dataset} & \textbf{Hparam} & \textbf{Randomness}  & \textbf{Default}\\
%     \midrule
%     \parbox[t]{2mm}{\multirow{11}{*}{\rotatebox[origin=c]{90}{\textsc{ColoredMNIST}}}} 
%      & $\xi$ & - & 0.1 \\
%      & $T$ & - & 1.0 \\
%      & $m_{in}$ & \text{Unif(-5.5, -5)} & -5.25 \\
%      & $m_{out}$ & \text{Unif(-4.5, -3.5)} & -4.0 \\
%      & $\gamma_1$ & \text{Unif(0.0001, 0.01)}  & 0.0025 \\
%      & $\gamma_2$ & \text{Unif(0.0001, 0.01)}  & 0.0025 \\
%      & $\eta_{p}$ & \text{Unif(0.001, 0.1)}  & 0.05 \\
%      & $\eta_{dg}$ & \text{Unif(0.001, 0.1)}  & 0.05 \\
%      & $\eta_{ood}$ & \text{Unif(0.001, 0.1)}  & 0.05 \\
%      \midrule
%      \parbox[t]{2mm}{\multirow{11}{*}{\rotatebox[origin=c]{90}{\textsc{PACS}}}}
%      & $\xi$ & - & 0.1 \\
%      & $T$ & - & 1.0 \\
%      & $m_{in}$ & \text{Unif(-11.0, -9.0)}  & -10.0 \\
%      & $m_{out}$ & \text{Unif(-9.0, -7.0)}  & -8.0 \\
%      & $\gamma_1$ & \text{Unif(0.0001, 0.01)}  & 0.0025 \\
%      & $\gamma_2$ & \text{Unif(15.0, 35.0)}  & 25.0 \\
%      & $\eta_{p}$ & \text{Unif(0.001, 0.1)}  & 0.05 \\
%      & $\eta_{dg}$ & \text{Unif(0.001, 0.1)}  & 0.05 \\
%      & $\eta_{ood}$ & \text{Unif(0.001, 0.1)}  & 0.05 \\
%      \midrule
%      \parbox[t]{2mm}{\multirow{11}{*}{\rotatebox[origin=c]{90}{\textsc{VLCS}}}} 
%      & $\xi$ & - & 0.1 \\
%      & $T$ & - & 1.0 \\
%      & $m_{in}$ & \text{Unif(-9.0, -7.0)}  & -8.0 \\
%      & $m_{out}$ & \text{Unif(-7.0, -5.0)}  & -6.0 \\
%      & $\gamma_1$ & \text{Unif(0.0001, 0.01)}  & 0.0025 \\
%      & $\gamma_2$ & \text{Unif(15.0, 35.0)}  & 25.0 \\
%      & $\eta_{p}$ & \text{Unif(0.001, 0.1)}  & 0.05 \\
%      & $\eta_{dg}$ & \text{Unif(0.001, 0.1)}  & 0.05 \\
%      & $\eta_{ood}$ & \text{Unif(0.001, 0.1)}  & 0.05 \\
%     \bottomrule
%     \end{tabular}
%     \label{tab:hyperparamesters}
% \end{table}

% \subsubsection{Datasets.}
% In our study, we assess the performance of our model on four popular datasets widely used in the field of domain generalization (DG): \textsc{ColoredMNIST} (3 domains, 70,000 samples, 2 classes), \textsc{PACS} (4 domains, 9,991 samples, 7 classes), and \textsc{VLCS} (4 domains, 10,729 samples, 5 classes).

% \textsc{ColoredMNIST} is a variant of the popular MNIST dataset of handwritten digits. It introduces color as a spurious feature, thereby creating three distinct domains for evaluating domain generalization capabilities. The three domains: [+90\%, +80\%, -90\%] are characterized by different levels of digit color and label correlations. The original 10 digits are split into two classes: digits from 0-4 are categorized with label 0, while digits from 5-9 receive label 1. Note that there is a 25\% manually injected error in the binary labels, which makes \textsc{ColoredMNIST} challenging for the domain generalization task.

% \textsc{PACS} dataset comprises images sourced from four discrete domains: Art Painting (A), Cartoon (C), Photo (P), and Sketch (S). Each domain offers a wide array of images showcasing diverse objects, scenes, and individuals. These images are categorized into seven different categories, namely dog, elephant, giraffe, guitar, horse, house, and person.

% \textsc{VLCS} is a collection of four well-established datasets
% commonly used in computer vision research: Caltech101 (C), LabelMe (L), SUN09 (S), and VOC2007 (V). These datasets, when brought together, offer an extensive variety of images across diverse
% contexts and subjects, making them an ideal test bed for assessing
% domain generalization capabilities. These images are categorized into five classes: person, dog, chair, car, and bird.

% Some examples of \textsc{ColoredMNIST}, \textsc{PACS}, and \textsc{VLCS} are shown in Figure \ref{fig:data-example}.

% \begin{figure*}
% \centering
% \begin{subfigure}{.3\textwidth}
%   \centering
%   \includegraphics[width=.9\linewidth]{images/coloredmnist.png}
%   \caption{\textsc{ColoredMNIST}}
%   \label{fig:coloredmnist}
% \end{subfigure}%
% \begin{subfigure}{.34\textwidth}
%   \centering
%   \includegraphics[width=.9\linewidth]{images/pacs.png}
%   \caption{\textsc{PACS}}
%   \label{fig:pacs}
% \end{subfigure}
% \begin{subfigure}{.34\textwidth}
%   \centering
%   \includegraphics[width=1\linewidth]{images/vlcs.png}
%   \caption{\textsc{VLCS}}
%   \label{fig:vlcs}
% \end{subfigure}
% \caption{Samples from each dataset. (a) \textsc{ColoredMNIST} domains are different levels of digit color and label correlation: +90\%, +80\%, and -90\%; (b) \textsc{PACS} domains are: Photo (P), Art Painting (A), Cartoon (C), and Sketch (S); (c) \textsc{VLCS} domains are: VOC2007 (V), LabelMe (L), Caltech101 (C), and SUN09 (S).}
% \label{fig:data-example}
% \end{figure*}

% \subsubsection{Baselines.}
% We compare the performance of our  with 4 state-of-the-art \textit{domain generalizations} methods: ERM \cite{vapnik1999nature}, IRM \cite{arjovsky2019invariant}, Mixup \cite{yan2020improve}, and MBDG \cite{robey2021model}. These experiments were conducted using the DomainBed \cite{gulrajani2020search} framework to ensure consistent assessment.

% \subsubsection{OOD Detection Methods.}
% To evaluate the performance of OOD detection, we employ four widely-used OOD detection methods: Maximum Softmax Probability (MSP) \cite{hendrycks2016baseline}, Energy-based Out-of-Distribution Detection (Energy) \cite{liu2020energy}, Deep Deterministic Uncertainty (DDU) \cite{mukhoti2021deep}, and One-Class Support Vector Machine (OCSVM) \cite{scholkopf1999support}. Each of these methods brings its unique approach to the problem, leveraging different aspects of the neural network's feature characteristics. As such, they each have their inherent strengths and potential limitations, providing us with a comprehensive understanding of our model's OOD detection performance.

% MSP (Maximum Softmax Probability) uses the softmax outputs of neural networks to identify OODs. Based on the assumption that neural networks are less confident when classifying OOD samples, hence, samples with lower maximum softmax probabilities are categorized as OOD.

% Energy (Energy-based Out-of-Distribution Detection) employs the output 'energies' of samples to detect OOD, with higher energy values indicating OOD samples. In comparison to MSP, Energy scores provide a closer representation of the input's probability density. As a result, they are less susceptible to the overconfidence issue.

% DDU (Deep Deterministic Uncertainty) detects OODs through estimated epistemic uncertainty (model uncertainty). The epistemic uncertainty of input is estimated by examining their feature-space density to the training data. Specifically, a per-class Gaussian mixture model (GMM) is fitted in the feature space, and at test time, the GMM is used to evaluate the test sample's marginal likelihood of its hidden representations in the feature space. 

% OCSVM (One-Class SVM) is a machine learning method specifically designed for anomaly detection. Unlike traditional SVMs that differentiate between two classes, OCSVM aims to identify patterns that conform to what it has seen during training (the "one class") and flag anything different as an outlier or anomaly. It achieves this by trying to maximize the distance between the data and the origin in the feature space, and then determining a decision boundary around the data. Anything that falls outside this boundary in the feature space is considered an anomaly. OCSVM is particularly useful in scenarios where "normal" data is abundant, but "anomalous" data is scarce or unavailable during training.

% \subsubsection{Evaluation Metrics.}
% To evaluate domain generalization performance, we simply report the classification accuracy. Meanwhile, to evaluate OOD detection performance, we use AUROC (Area Under the Receiver Operating Characteristic Curve) and AUPR (Area Under the Precision-Recall
% Curve). AUROC is a commonly used metric for evaluating the effectiveness of binary classification models. It measures the model's capacity to differentiate between positive and negative classes by computing the area under the ROC curve. This value can range from 0 to 1, with a perfect model having an AUROC of 1 and a random model having an AUROC of 0.5. The AUPR is a metric used to evaluate the performance of a classification model, especially in imbalanced datasets where one class significantly outnumbers the other. The precision-recall curve plots precision against recall for different threshold values. The AUPR calculates the area under this curve, providing a single value that captures the model's ability to correctly classify the positive class across various thresholds. A higher AUPR value indicates better model performance, with a maximum value of 1. In cases of imbalanced datasets, AUPR is often preferred over the more common AUROC because it focuses specifically on the performance with respect to the positive, or minority class. In the paper, the AUPR values we reported are the AUPR-out which treats OODs as positive samples.
% Note that the results reported in the paper are the mean and standard error across trials and all OOD class choices. And for the OOD detection performance evaluation, the AUROC and AUPR values are further averaged across all test domain selections to save space.



% \subsection{Additional Experimental Results.}
% In Table 1, we present the OOD detection performance of \sysname{} in comparison to several common domain generalization baselines across three datasets, utilizing the AUROC as our evaluation metric. However, relying solely on the AUROC can be misleading, as it doesn't factor in class imbalances. To provide a more comprehensive evaluation, in Table \ref{tab:aupr-summary}, we report the corresponding AUPR, considering OODs as positive instances. These results reveal that, while \sysname{} consistently outperforms all baselines by a large margin, the AUPR values tend to be considerably lower than their AUROC counterparts. This discrepancy underscores the inherent difficulty in accurately identifying semantic OODs. Given that both OODs and InD test samples originate from the same test domain, it poses a significant challenge for an OOD detector to simultaneously achieve high precision and recall in detecting these semantic OODs in an unseen test domain. In real-world scenarios, based on the chosen OOD score threshold, one might anticipate a high false positive rate across all three datasets.


% \begin{table*}[!t]
% \centering
% % \setlength\tabcolsep{5pt}
% % \scriptsize
% \caption{Performance Evaluation: All AUPR values represent the average across all trials, OOD class selections, and test domains. Top results are highlighted in \textbf{bold}.}
% \begin{tabular}{c|l|c|c|c|c|c}
% \toprule
% \multirow{3}{*}{Data} &  & \multicolumn{5}{c}{\textbf{OOD Detection, AUPR}} \\
% \cmidrule{3-7}
% & & \multicolumn{5}{c}{OOD Detection Algorithms} \\
% \midrule
% & Methods & MSP    & Energy & DDU & OCSVM & Avg\\ 
% \cmidrule{2-7}
% \parbox[t]{2mm}{\multirow{5}{*}{\rotatebox[origin=c]{90}{\textsc{\scriptsize ColoredMNIST}}}} 
% & ERM    & 09.83 $\pm$ 0.39 & 10.47 $\pm$ 0.04 & 09.13 $\pm$ 0.10 & 10.72 $\pm$ 0.38 & 10.04 \\
% & IRM    & 10.52 $\pm$ 1.07 & 10.14 $\pm$ 0.65 & 09.42 $\pm$ 0.61 & 11.15 $\pm$ 0.10 & 10.31 \\
% & Mixup  & 10.43 $\pm$ 0.62 & 09.97 $\pm$ 0.36 & 09.09 $\pm$ 0.04 & 10.94 $\pm$ 0.75 & 10.11 \\
% & MBDG   & 14.17 $\pm$ 2.52 & 15.16 $\pm$ 2.58 & 08.24 $\pm$ 0.27 & 14.14 $\pm$ 1.74 & 12.92 \\
% \cmidrule{2-7}
% & Ours   & \textbf{57.43} $\pm$ 0.35 & \textbf{57.37} $\pm$ 0.36 & \textbf{42.47} $\pm$ 0.89 & \textbf{55.28} $\pm$ 0.25 & \textbf{53.14} \\
% \midrule
%  & Methods & MSP    & Energy & DDU & OCSVM & Avg\\
% \cmidrule{2-7}
% \parbox[t]{2mm}{\multirow{5}{*}{\rotatebox[origin=c]{90}{\textsc{PACS}}}} 
% & ERM    & 32.64 $\pm$ 3.44 & 38.96 $\pm$ 3.36 & 25.06 $\pm$ 3.56 & 19.87 $\pm$ 0.92 & 29.13 \\
% & IRM    & 35.20 $\pm$ 7.45 & 42.14 $\pm$ 7.63 & 22.28 $\pm$ 3.58 & 23.84 $\pm$ 3.22 & 30.86 \\
% & Mixup  & 32.70 $\pm$ 6.77 & 35.22 $\pm$ 7.11 & 33.54 $\pm$ 2.46 & 17.56 $\pm$ 5.11 & 29.76 \\
% & MBDG   & 31.93 $\pm$ 4.38 & 36.34 $\pm$ 4.95 & 22.39 $\pm$ 5.24 & 22.03 $\pm$ 1.90 & 28.17 \\
% \cmidrule{2-7}
% & Ours   & \textbf{57.26} $\pm$ 0.51 & \textbf{57.70} $\pm$ 0.50 & \textbf{57.30} $\pm$ 0.60 & \textbf{43.37} $\pm$ 0.66 & \textbf{53.91} \\
% \midrule
%  & Methods & MSP    & Energy & DDU & OCSVM & Avg\\
% \cmidrule{2-7}
% \parbox[t]{2mm}{\multirow{5}{*}{\rotatebox[origin=c]{90}{\textsc{VLCS}}}} 
% & ERM    & 24.52 $\pm$ 11.83 & 27.63 $\pm$ 12.34 & 21.46 $\pm$ 7.57 & 08.82 $\pm$ 2.25 & 20.60 \\
% & IRM    & 23.73 $\pm$ 11.54 & 27.82 $\pm$ 12.28 & 20.75 $\pm$ 8.00 & 09.69 $\pm$ 2.35 & 20.49 \\
% & Mixup  & 21.60 $\pm$ 10.69 & 26.14 $\pm$ 10.55 & 26.63 $\pm$ 4.60 & 10.31 $\pm$ 2.95 & 21.17 \\
% & MBDG   & 15.92 $\pm$ 05.25 & 21.16 $\pm$ 07.42 & 18.66 $\pm$ 0.91 & 08.34 $\pm$ 2.53 & 16.02 \\
% \cmidrule{2-7}
% & Ours   & \textbf{47.40} $\pm$ 02.60 & \textbf{48.04} $\pm$ 02.23 & \textbf{48.73} $\pm$ 1.73 & \textbf{39.42} $\pm$ 3.43 & \textbf{45.90} \\
% \bottomrule
% \end{tabular}
% \label{tab:aupr-summary}
% \end{table*}


% In Tables \ref{tab:ood-details-1}, \ref{tab:ood-details-2}, and \ref{tab:ood-details-3}, we report the detailed AUROC values for each test domain. From these results, it is evident that \sysname{} consistently stands out, delivering superior performance across the majority of configurations.

% \begin{table*}[!t]
% \centering
% % \setlength\tabcolsep{5pt}
% \scriptsize
% \caption{\textsc{ColoredMNIST} Performance Evaluation Details: The AUROC values are the average across all trials, OOD class selections. Top results are highlighted in \textbf{bold}.}
% \begin{tabular}{c|l|c|c|c|c}
% \toprule
% \multirow{3}{*}{Data} &  & \multicolumn{4}{c}{\textbf{OOD Detection, AUROC}} \\
% \cmidrule{3-6}
% & & \multicolumn{4}{c}{OOD Detection Algorithms}  \\
% \cmidrule{1-6}
% & Methods & MSP    & Energy & DDU & OCSVM  \\ 
% \cmidrule{2-6}
% \parbox[t]{2mm}{\multirow{5}{*}{\rotatebox[origin=c]{90}{+90\%}}} 
% & ERM    & 49.72 $\pm$ 2.29 & 50.54 $\pm$ 2.74 & 50.54 $\pm$ 5.63 & 53.17 $\pm$ 2.80 \\
% & IRM    & 57.20 $\pm$ 2.21 & 51.94 $\pm$ 6.06 & 52.36 $\pm$ 2.05 & 53.17 $\pm$ 0.49 \\
% & Mixup  & 53.00 $\pm$ 1.74 & 49.50 $\pm$ 2.45 & 53.20 $\pm$ 4.43 & 55.84 $\pm$ 1.90 \\
% & MBDG   & 62.94 $\pm$ 3.60 & 66.34 $\pm$ 4.92 & 71.54 $\pm$ 8.99 & 56.72 $\pm$ 4.34 \\
% \cmidrule{2-6}
% & Ours   & \textbf{86.19} $\pm$ 2.13 & \textbf{86.28} $\pm$ 2.09 & \textbf{79.61} $\pm$ 3.24 & \textbf{76.95} $\pm$ 2.86  \\
% \midrule
% \parbox[t]{2mm}{\multirow{5}{*}{\rotatebox[origin=c]{90}{+80\%}}} 
% & ERM    & 50.78 $\pm$ 1.72 & 50.38 $\pm$ 3.49 & 48.74 $\pm$ 5.79 & 51.10 $\pm$ 2.17  \\
% & IRM    & 49.16 $\pm$ 1.57 & 48.87 $\pm$ 3.66 & 48.06 $\pm$ 3.76 & 52.51 $\pm$ 3.03  \\
% & Mixup  & 49.50 $\pm$ 2.08 & 51.88 $\pm$ 2.27 & 52.08 $\pm$ 3.44 & 52.65 $\pm$ 3.09  \\
% & MBDG   & 65.52 $\pm$ 5.91 & 64.89 $\pm$ 5.61 & 69.70 $\pm$ 4.15 & 54.26 $\pm$ 4.25  \\
% \cmidrule{2-6}
% & Ours   & \textbf{81.58} $\pm$ 2.67 & \textbf{80.88} $\pm$ 2.46 & \textbf{72.48} $\pm$ 5.30 & \textbf{70.89} $\pm$ 3.08  \\
% \midrule
% \parbox[t]{2mm}{\multirow{5}{*}{\rotatebox[origin=c]{90}{-90\%}}} 
% & ERM    & 46.28 $\pm$ 2.09 & 50.26 $\pm$ 3.60 & 57.23 $\pm$ 5.34 & 51.11 $\pm$ 2.19  \\
% & IRM    & 46.98 $\pm$ 1.55 & 46.90 $\pm$ 2.39 & 50.05 $\pm$ 3.54 & 53.28 $\pm$ 1.21  \\
% & Mixup  & 48.26 $\pm$ 1.17 & 47.55 $\pm$ 3.22 & 51.09 $\pm$ 2.95 & 51.20 $\pm$ 3.66  \\
% & MBDG   & 46.93 $\pm$ 4.22 & 48.59 $\pm$ 3.11 & 47.46 $\pm$ 6.35 & 51.86 $\pm$ 3.98  \\
% \cmidrule{2-6}
% & Ours   & \textbf{77.67} $\pm$ 1.97 & \textbf{77.53} $\pm$ 1.80 & \textbf{72.62} $\pm$ 3.66 & \textbf{71.24} $\pm$ 4.96  \\
% \bottomrule
% \end{tabular}
% \label{tab:ood-details-1}
% \end{table*}



% \begin{table*}[!t]
% \centering
% % \setlength\tabcolsep{5pt}
% \scriptsize
% \caption{\textsc{PACS} Performance Evaluation Details: The AUROC values are the average across all trials, OOD class selections. Top results are highlighted in \textbf{bold}.}
% \begin{tabular}{c|l|c|c|c|c}
% \toprule
% \multirow{3}{*}{Data} &  & \multicolumn{4}{c}{\textbf{OOD Detection, AUROC}} \\
% \cmidrule{3-6}
% & & \multicolumn{4}{c}{OOD Detection Algorithms}  \\
% \midrule
% & Methods & MSP    & Energy & DDU & OCSVM  \\ 
% \cmidrule{2-6}
% \parbox[t]{2mm}{\multirow{5}{*}{\rotatebox[origin=c]{90}{Art Painting}}} 
% & ERM    & 79.79 $\pm$ 4.28 & 80.00 $\pm$ 5.81 & 53.70 $\pm$ 7.56 & 50.15 $\pm$ 5.27  \\
% & IRM    & 77.08 $\pm$ 5.31 & 78.05 $\pm$ 7.22 & 48.38 $\pm$ 12.87 & 58.81 $\pm$ 4.86  \\
% & Mixup  & 75.17 $\pm$ 5.46 & 75.14 $\pm$ 6.07 & 70.06 $\pm$ 3.98 & 38.53 $\pm$ 3.25  \\
% & MBDG   & 75.70 $\pm$ 1.86 & 75.62 $\pm$ 4.02 & 48.35 $\pm$ 10.66 & \textbf{61.09} $\pm$ 6.14  \\
% \cmidrule{2-6}
% & Ours   & \textbf{83.02} $\pm$ 3.52 & \textbf{84.50} $\pm$ 4.95 & \textbf{81.15} $\pm$ 4.67 & 52.47 $\pm$ 7.69  \\
% \midrule
% \parbox[t]{2mm}{\multirow{5}{*}{\rotatebox[origin=c]{90}{Cartoon}}} 
% & ERM    & 73.83 $\pm$ 2.55 & 74.90 $\pm$ 4.06 & 65.79 $\pm$ 14.52 & 44.38 $\pm$ 16.92  \\
% & IRM    & 69.06 $\pm$ 8.36 & 72.18 $\pm$ 9.50 & 64.42 $\pm$ 7.50 & 45.96 $\pm$ 12.59  \\
% & Mixup  & 66.83 $\pm$ 4.79 & 64.28 $\pm$ 4.25 & 75.01 $\pm$ 5.61 & 29.09 $\pm$ 7.13  \\
% & MBDG   & 68.72 $\pm$ 4.69 & 69.28 $\pm$ 5.37 & 63.72 $\pm$ 0.68 & 46.63 $\pm$ 4.91  \\
% \cmidrule{2-6}
% & Ours   & \textbf{80.32} $\pm$ 2.57 & \textbf{84.16} $\pm$ 2.59 & \textbf{83.59} $\pm$ 4.45 & \textbf{64.85} $\pm$ 9.77  \\
% \midrule
% \parbox[t]{2mm}{\multirow{5}{*}{\rotatebox[origin=c]{90}{Photo}}} 
% & ERM    & 81.83 $\pm$ 7.00 & 83.22 $\pm$ 6.74 & 59.06 $\pm$ 11.86 & 51.73 $\pm$ 4.91  \\
% & IRM    & 92.05 $\pm$ 0.38 & 93.41 $\pm$ 0.79 & 51.14 $\pm$ 12.63 & \textbf{63.61} $\pm$ 9.24  \\
% & Mixup  & 87.13 $\pm$ 1.69 & 85.21 $\pm$ 2.78 & 64.13 $\pm$ 22.94 & 39.33 $\pm$ 24.24  \\
% & MBDG   & 84.67 $\pm$ 4.76 & 85.37 $\pm$ 5.06 & 69.04 $\pm$ 7.78 & 46.25 $\pm$ 2.10  \\
% \cmidrule{2-6}
% & Ours   & \textbf{93.31} $\pm$ 2.78 & \textbf{94.87} $\pm$ 2.82 & \textbf{93.75} $\pm$ 2.99 & 54.68 $\pm$ 6.24  \\
% \midrule
% \parbox[t]{2mm}{\multirow{5}{*}{\rotatebox[origin=c]{90}{Sketch}}} 
% & ERM    & 76.71 $\pm$ 4.48 & 82.38 $\pm$ 5.30 & 43.82 $\pm$ 1.94 & 51.89 $\pm$ 4.83  \\
% & IRM    & 74.02 $\pm$ 0.59 & 80.64 $\pm$ 1.95 & 37.98 $\pm$ 8.25 & 57.32 $\pm$ 1.12  \\
% & Mixup  & 69.68 $\pm$ 2.70 & 71.94 $\pm$ 0.63 & 66.88 $\pm$ 6.33 & 34.22 $\pm$ 10.10  \\
% & MBDG   & 76.64 $\pm$ 2.01 & 83.76 $\pm$ 1.87 & 34.47 $\pm$ 8.42 & \textbf{72.03} $\pm$ 9.26  \\
% \cmidrule{2-6}
% & Ours   & \textbf{82.45} $\pm$ 1.87 & \textbf{88.02} $\pm$ 2.56 & \textbf{84.09} $\pm$ 3.71 & 62.82 $\pm$ 12.30  \\
% \bottomrule
% \end{tabular}
% \label{tab:ood-details-2}
% \end{table*}


% \begin{table*}[!t]
% \centering
% % \setlength\tabcolsep{5pt}
% \scriptsize
% \caption{\textsc{VLCS} Performance Evaluation Details: The AUROC values are the average across all trials, OOD class selections. Top results are highlighted in \textbf{bold}.}
% \begin{tabular}{c|l|c|c|c|c}
% \toprule
% \multirow{3}{*}{Data} &  & \multicolumn{4}{c}{\textbf{OOD Detection, AUROC}} \\
% \cmidrule{3-6}
% & & \multicolumn{4}{c}{OOD Detection Algorithms}  \\
% \cmidrule{1-6}
% & Methods & MSP    & Energy & DDU & OCSVM  \\ 
% \cmidrule{2-6}
% \parbox[t]{2mm}{\multirow{5}{*}{\rotatebox[origin=c]{90}{Caltech101}}} 
% & ERM    & 92.01 $\pm$ 4.20 & 93.62 $\pm$ 3.00 & 82.13 $\pm$ 9.01 & 19.34 $\pm$ 12.10  \\
% & IRM    & 89.45 $\pm$ 7.11 & 90.44 $\pm$ 6.40 & 80.53 $\pm$ 7.60 & 16.26 $\pm$ 9.22  \\
% & Mixup  & 89.60 $\pm$ 1.34 & 90.02 $\pm$ 0.37 & 81.26 $\pm$ 7.79 & 14.62 $\pm$ 0.56  \\
% & MBDG   & 83.00 $\pm$ 6.66 & 87.46 $\pm$ 5.02 & 61.02 $\pm$ 3.56 & 75.58 $\pm$ 1.30  \\
% \cmidrule{2-6}
% & Ours   & \textbf{93.34} $\pm$ 4.39 & \textbf{94.54} $\pm$ 2.88 & \textbf{95.62} $\pm$ 2.63 & \textbf{90.00} $\pm$ 3.83  \\
% \midrule
% \parbox[t]{2mm}{\multirow{5}{*}{\rotatebox[origin=c]{90}{LabelMe}}} 
% & ERM    & 71.49 $\pm$ 3.75 & 73.24 $\pm$ 2.62 & 37.30 $\pm$ 8.34 & 46.96 $\pm$ 17.42  \\
% & IRM    & 71.82 $\pm$ 3.68 & 73.63 $\pm$ 4.31 & 37.68 $\pm$ 5.26 & 45.38 $\pm$ 9.26  \\
% & Mixup  & 66.82 $\pm$ 10.78 & 67.34 $\pm$ 12.70 & 52.88 $\pm$ 20.02 & 28.06 $\pm$ 14.97  \\
% & MBDG   & 71.17 $\pm$ 5.37 & 74.20 $\pm$ 4.82 & 41.32 $\pm$ 8.79 & 58.48 $\pm$ 14.13  \\
% \cmidrule{2-6}
% & Ours   & \textbf{80.52} $\pm$ 8.14 & \textbf{83.28} $\pm$ 10.02 & \textbf{84.30} $\pm$ 9.95 & \textbf{61.20} $\pm$ 4.89  \\
% \midrule
% \parbox[t]{2mm}{\multirow{5}{*}{\rotatebox[origin=c]{90}{Sun09}}} 
% & ERM    & 54.97 $\pm$ 1.75 & 57.48 $\pm$ 1.95 & 60.26 $\pm$ 1.68 & 33.54 $\pm$ 2.38  \\
% & IRM    & 56.53 $\pm$ 3.57 & 62.58 $\pm$ 0.62 & 62.62 $\pm$ 6.77 & 32.98 $\pm$ 8.14  \\
% & Mixup  & 53.60 $\pm$ 6.39 & 57.02 $\pm$ 3.86 & 63.42 $\pm$ 6.52 & 29.39 $\pm$ 6.23  \\
% & MBDG   & 56.04 $\pm$ 11.12 & 65.11 $\pm$ 6.70 & 54.96 $\pm$ 3.64 & 62.94 $\pm$ 1.90  \\
% \cmidrule{2-6}
% & Ours   & \textbf{62.98} $\pm$ 1.61 & \textbf{69.56} $\pm$ 1.90 & \textbf{76.12} $\pm$ 5.20 & \textbf{69.59} $\pm$ 4.00  \\
% \midrule
% \parbox[t]{2mm}{\multirow{5}{*}{\rotatebox[origin=c]{90}{VOC2007}}} 
% & ERM    & 59.72 $\pm$ 8.13 & 63.81 $\pm$ 3.74 & 52.46 $\pm$ 22.50 & 42.00 $\pm$ 23.96  \\
% & IRM    & 58.68 $\pm$ 7.69 & 63.52 $\pm$ 8.60 & 47.04 $\pm$ 22.12 & 46.15 $\pm$ 23.57  \\
% & Mixup  & 50.78 $\pm$ 1.10 & 58.34 $\pm$ 1.19 & 41.92 $\pm$ 22.15 & 49.03 $\pm$ 26.46  \\
% & MBDG   & 52.18 $\pm$ 3.28 & 60.78 $\pm$ 5.91 & 47.40 $\pm$ 4.91 & \textbf{54.12} $\pm$ 26.16  \\
% \cmidrule{2-6}
% & Ours   & \textbf{63.33} $\pm$ 2.29 & \textbf{67.16} $\pm$ 1.57 & \textbf{64.50} $\pm$ 16.30 & 52.22 $\pm$ 15.13  \\
% \bottomrule
% \end{tabular}
% \label{tab:ood-details-3}
% \end{table*}


% \subsection{Additional Ablation Study Results.}
% In Table 2, we presented the average AUROC values for each setting and observed that both $R_{DG}$ and $R_{OOD}$ contribute to \sysname{}'s final OOD detection performance. These findings are further complemented by Table \ref{tab:ablation-details}, where the corresponding average AUPR is reported. Clearly, the trends observed in AUPR seamlessly echo those from the AUROC metric. Across all datasets, it's evident that the full version of \sysname{} consistently delivers the best performance in terms of average AUPR.

% \begin{table*}[!t]
% \centering
% % \setlength\tabcolsep{5pt}
% % \scriptsize
% \caption{Ablation Study Performance Evaluation: The reported AUPR values represent the average across all trials, OOD class selections, and test domains. The top-performing results are highlighted in \textbf{bold}.}
% \begin{tabular}{c|l|c|c|c|c|c}
% \toprule
% Data & Settings & MSP & Energy & DDU & OCSVM & Avg \\
% \midrule
% \parbox[t]{2mm}{\multirow{3}{*}{\rotatebox[origin=c]{90}{\textsc{\textsc{\scriptsize CMNIST}}}}} 
% & \sysname{} w/o $R_{OOD}$\&$R_{DG}$         & 09.83 $\pm$ 0.39 & 10.47 $\pm$ 0.04 & 09.13 $\pm$ 0.10 & 10.72 $\pm$ 0.38 & 10.04 \\
% & \sysname{} w/o $R_{OOD}$    & 39.11 $\pm$ 1.42 & 39.25 $\pm$ 1.10 & 26.87 $\pm$ 0.31 & 41.54 $\pm$ 2.28 & 36.69 \\
% & \sysname{} (full) & \textbf{57.43} $\pm$ 0.35 & \textbf{57.37} $\pm$ 0.36 & \textbf{42.47} $\pm$ 0.89 & \textbf{55.28} $\pm$ 0.25 & \textbf{53.14} \\
% \midrule
% \parbox[t]{2mm}{\multirow{3}{*}{\rotatebox[origin=c]{90}{\textsc{\textsc{PACS}}}}} 
% & \sysname{} w/o $R_{OOD}$\&$R_{DG}$         & 32.64 $\pm$ 3.44 & 38.96 $\pm$ 3.36 & 25.06 $\pm$ 3.56 & 19.87 $\pm$ 0.92 & 29.13 \\
% & \sysname{} w/o $R_{OOD}$    & 34.93 $\pm$ 5.57 & 41.3 $\pm$ 6.03 & 39.44 $\pm$ 6.96 & \textbf{57.50} $\pm$ 2.59 & 43.29 \\
% & \sysname{} (full) & \textbf{57.26} $\pm$ 0.51 & \textbf{57.7} $\pm$ 0.50 & \textbf{57.30} $\pm$ 0.60 & 43.37 $\pm$ 0.66 & \textbf{53.91} \\
% \midrule
% \parbox[t]{2mm}{\multirow{3}{*}{\rotatebox[origin=c]{90}{\textsc{\textsc{VLCS}}}}} 
% & \sysname{} w/o $R_{OOD}$\&$R_{DG}$         & 24.52 $\pm$ 11.83 & 27.63 $\pm$ 12.34 & 21.46 $\pm$ 7.57 & 08.82 $\pm$ 2.25 & 20.60 \\
% & \sysname{} w/o $R_{OOD}$    & 26.34 $\pm$ 13.28 & 30.98 $\pm$ 11.52 & 28.32 $\pm$ 4.57 & \textbf{39.43} $\pm$ 2.17 & 31.27 \\
% & \sysname{} (full) & \textbf{47.40} $\pm$ 02.60 & \textbf{48.04} $\pm$ 02.23 & \textbf{48.73} $\pm$ 1.73 & 39.42 $\pm$ 3.43 & \textbf{45.90} \\
% \bottomrule
% \end{tabular}
% \label{tab:ablation-details}
% \end{table*}

% \subsection{Feature Space Regularization versus Output Space Regularization.}
% In this paper, the semantic $G$-invariance is learned through feature space regularization. Specifically, we employ the domain generalization regularization term $R_{DG}$ to enforce the semantic between $(\mathbf{x}^{e},y)$ and the random domain counterpart $(\mathbf{x}^{e'},y)$ in the feature space. One might wonder why we prioritize the feature space over the output space for learning semantic $G$-invariance. The primary reason is that the feature space representations contain richer information than the final outputs. As highlighted by recent neural network interpretation studies \cite{zhou2018interpreting,rauker2023toward}, deeper layers in a neural network tend to capture increasingly complex concepts. As for the output space, constrained by its feature dimension, typically represents high-level conceptual semantics, thereby limiting its representational capacity. Furthermore, OOD can take many forms, each with unique characteristics. Some OODs might exhibit only subtle deviations from the in-distribution data. To identify such nuanced differences, it becomes imperative to leverage features with higher representational capacity.

% To provide a comparative perspective, we compare \sysname{}, which employs feature space regularization, against a model where the $R_{DG}$ term is substituted with output space regularization. Their respective t-SNE visualizations, derived from the PACS dataset with "Art Painting" as the test domain and class 6 as OODs, are presented in Figure \ref{fig:reg-compare}. It is evident that the feature space regularization approach provides clearer boundaries for each class cluster. Moreover, the OOD samples (pink points) mostly lie in the middle with less overlapping with InD clusters.


% \begin{figure*}[!t]
% \centering
%     \begin{subfigure}[b]{0.65\textwidth}
%        \includegraphics[width=1\linewidth]{images/output_space_regularization.png}
%        \caption{Output space regularization}
%        \label{fig:Ng1} 
%     \end{subfigure}
    
%     \begin{subfigure}[b]{0.65\textwidth}
%        \includegraphics[width=1\linewidth]{images/feature_space_regularization.png}
%        \caption{Feature space regularization}
%        \label{fig:Ng2}
%     \end{subfigure}
    
%     \caption{Comparison of t-SNE plots for latent features of models using output space regularization versus feature space regularization. These plots are generated on the \textsc{PACS} dataset, with "Art Painting" as the test domain. Class 6 (pink) is the designated OOD class.}
% \label{fig:reg-compare}
% \end{figure*}

% \subsection{Proof}
